# Supplementary material for: Limitations and Biases in Facial Landmark Detection -- An Empirical Study on Older Adults with Dementia
Source: arXiv:1905.07446 source file (2019-05-17)
Supplement: Supplementary file 1 [file Supplementary_Materials.pdf]

# Supplementary Material

## 1. Implementation Details

In this section we provide the details of different methods used in our evaluation and how different models were re-trained/fine-tuned.

### 1.1. Active Appearance Models (AAM)

To re-train the AAM model, the implementation by MENPO Group (https://github.com/menpo/menpo) was used. Training data was cropped around the face region and the training landmarks were re-scaled so that the diagonal of the images are 150 pixels. Next, SIFT features were extracted from the images at three scales (0.25, 0.5, and 1.0) and were used to train a Holistic AAM with max appearance components of 200, and max shape components of 20. During inference, a Lucas Kanade Fitter was used with 1, 5, 15 shape components and 15, 100, 150 appearance components, respectively for each of the three scales.

### 1.2. Constrained Local Neural Field (CLNF)

To re-train the Constrained Local Neural Field (CLNF) model, the implementation provided by the authors (https://github.com/TadasBaltrusaitis) was used. First, the face images and ground truth facial landmarks were scaled to 0.25, 0.35, 0.5, 1.0 times the original scale and used to train the Local Neural Field patch experts. Then, the facial landmarks were aligned and re-scaled to the same size according to pupil to pupil distance and principal component analysis was performed to create the shape component.

### 1.3. Coarse-to-Fine Shape Searching (CFSS)

To re-train the CFSS model, the original implementation by the authors (https://github.com/zhusz/CVPR15-CFSS) was used. Training data was cropped over the face region, augmented ten times by rotating to a random angle within 45 degrees. Then, Histogram of Oriented Gradients (HOG) features of the augmented images were used for training a decision tree to align the shapes to the mean shape. Next, a regressor was trained to estimate the current pose of an image by sampling from a probability distribution of candidate face poses. Finally, a Support Vector Machine (SVM) was used to learn the probability distribution of the candidate faces given the SIFT features around the current pose. The regression of the pose and the probability inference were cascaded a total of three times.

### 1.4. Face Alignment Network (FAN)

For fine-tuning the FAN model, the original implementation by the authors (https://github.com/1adrianb/face-alignment) was used. The training images and landmarks were cropped around the face by a square bounding box proportional to the size (width + height) of the ground truth bounding box. The training data was re-scaled to 64 x 64. The 68 landmark points were used to generate 68 heatmaps, each corresponding to one landmark. The images were augmented with rotation of up to 10 degrees, horizontal flip, lowered resolution, and random hue. The prepared data was then used to fine-tune the FAN with four stacked hourglass blocks, with only the last hourglass unfrozen. The fine-tuning starts with learning rate of 2.5e-4, and is scaled down by a factor of 0.2 with the patience of 3 when facing a plateau in the loss curve.

### 1.5. Mnemonic Descent Method (MDM)

To evaluate the Mnemonic Descent Method (MDM) model, the original implementation by the authors (https://github.com/trigeorgis/mdm) was used.

### 1.6. Position Map Regression Network (PRNet)

The original implementation of the PRNet model (https://github.com/YadiraF/PRNet) by the authors was used in our evaluation.

## 2. Additional results

The results obtained for healthy (H) and dementia (D) subsets of $T_f$ and $T_p$ by individual methods explored in Experiments 1-4 are presented here separately for each region of the face.

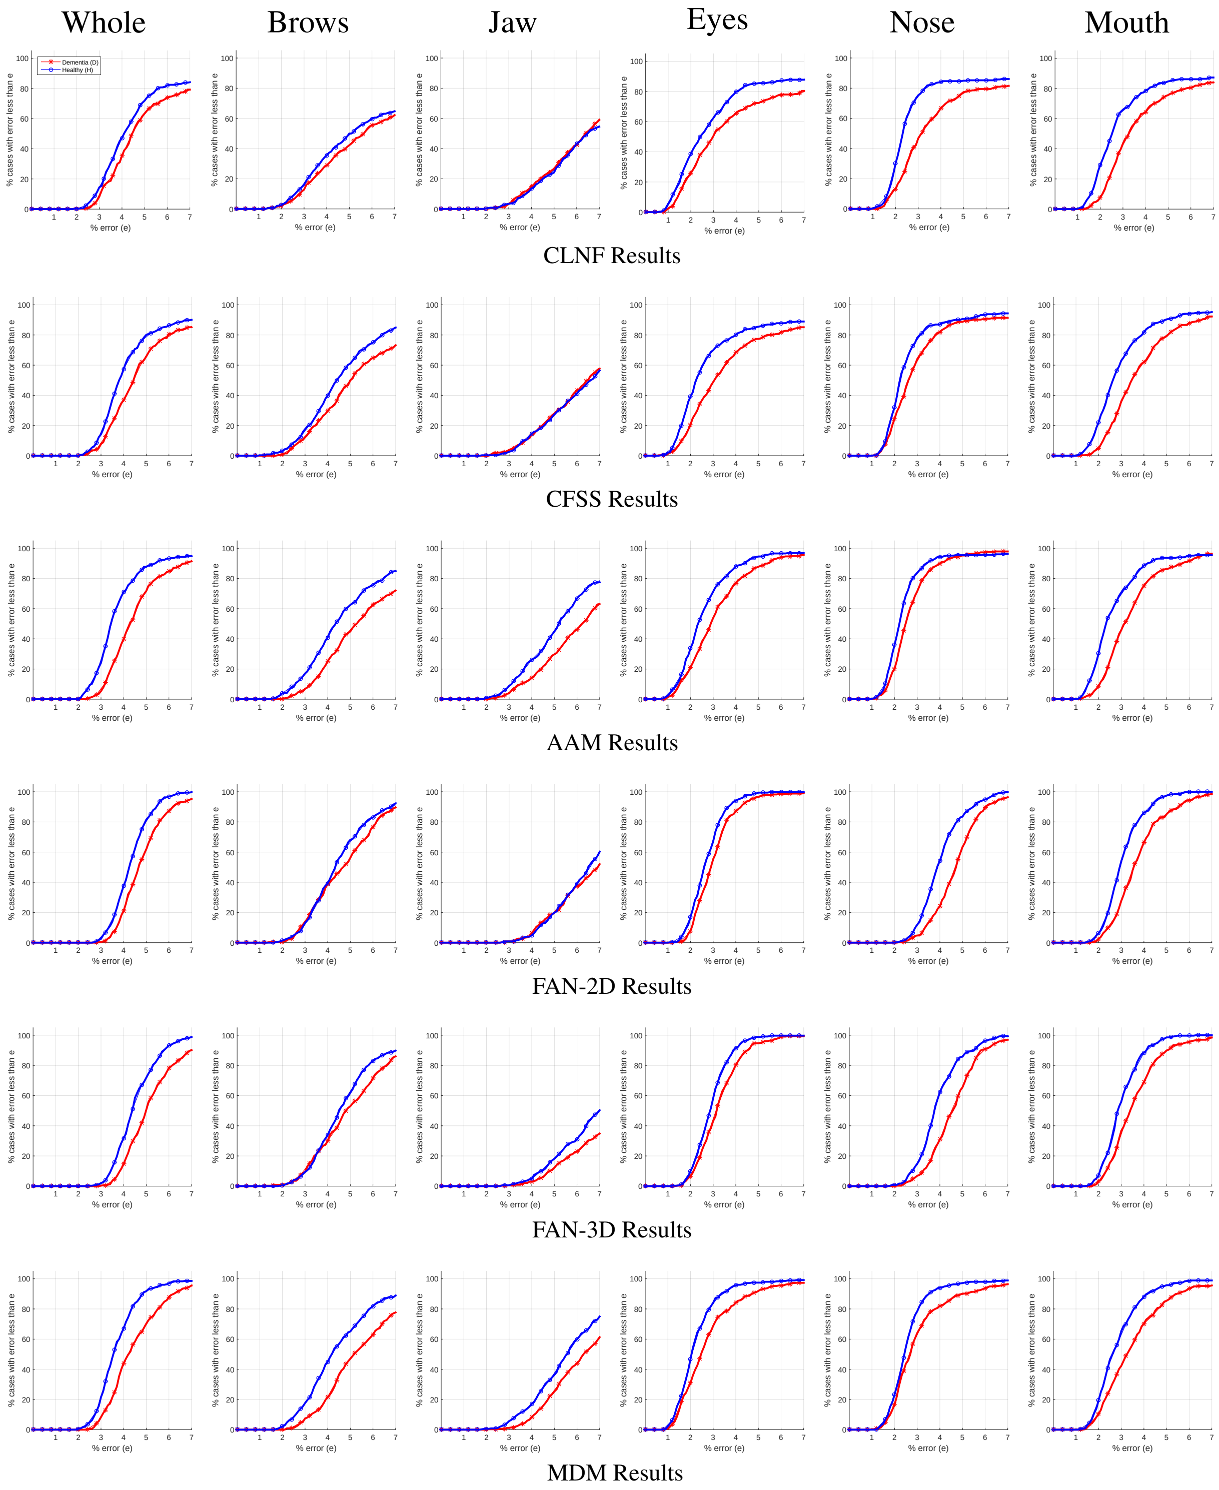

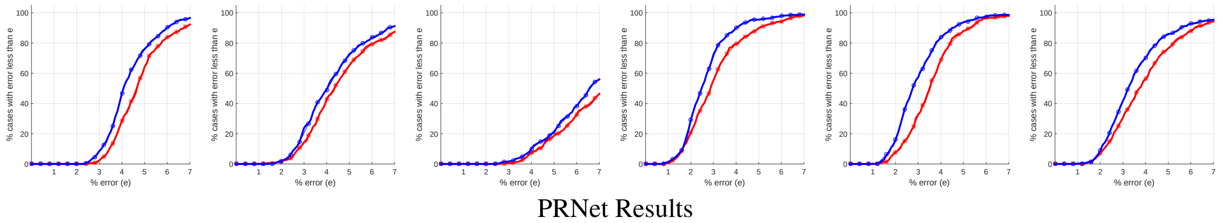


Figure 1: Experiment 1: Comparison of the convergence curves obtained on healthy subset (H) and dementia subset (D) of $T_f$ using off-the-shelf versions of seven methods: CLNF, CFSS, AAM, FAN-2D, FAN-3D, MDM, and PRNet.

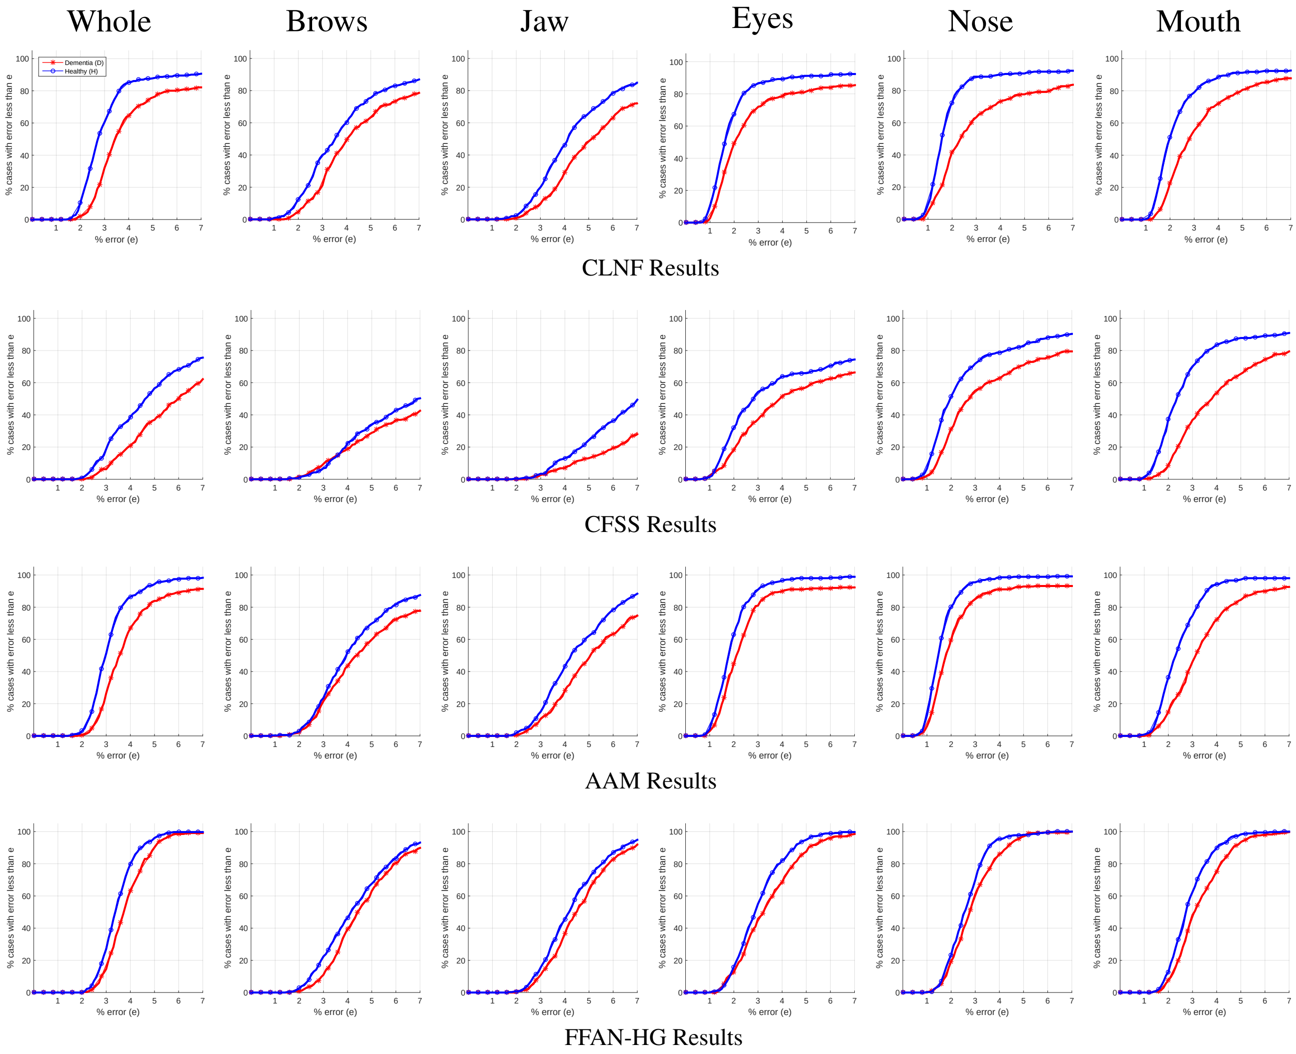


Figure 2: Experiment 2: Comparison of the convergence curves obtained on healthy subset (H) and dementia subset (D) of $T_f$ with fine-tuned/re-trained versions of four methods CLNF, CFSS, AAM, and FFAN-HG with $T_f$.

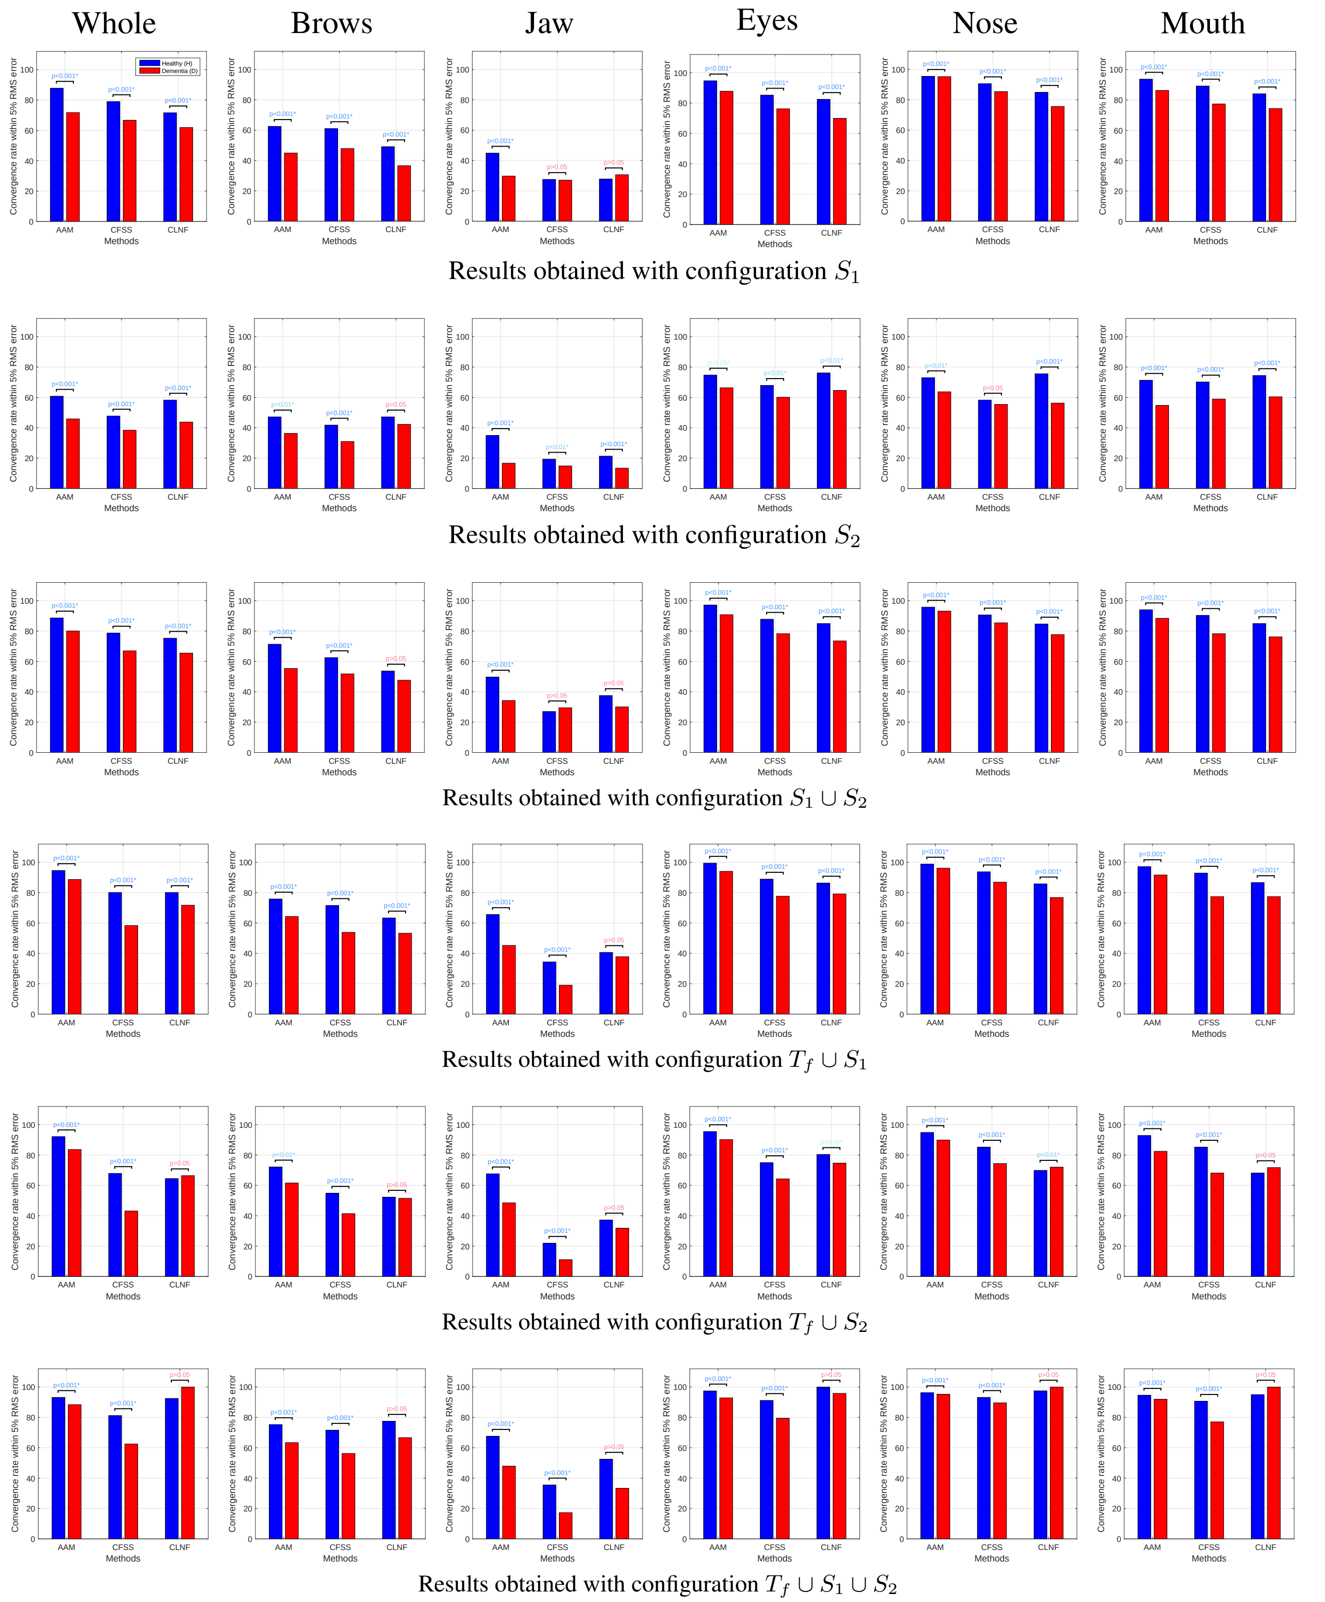


Figure 3: Experiment 3: Comparison of convergence percentage within 5% tolerance of RMS fitting error obtained on healthy subset (H) and dementia subset (D) of $T_f$ using various versions of three methods AAM, CFSS, and CLNF trained on configurations $S_1, S_2, S_1 \cup S_2, T_f \cup S_1,\ T_f \cup S_2,\ T_f \cup S_1 \cup S_2$.

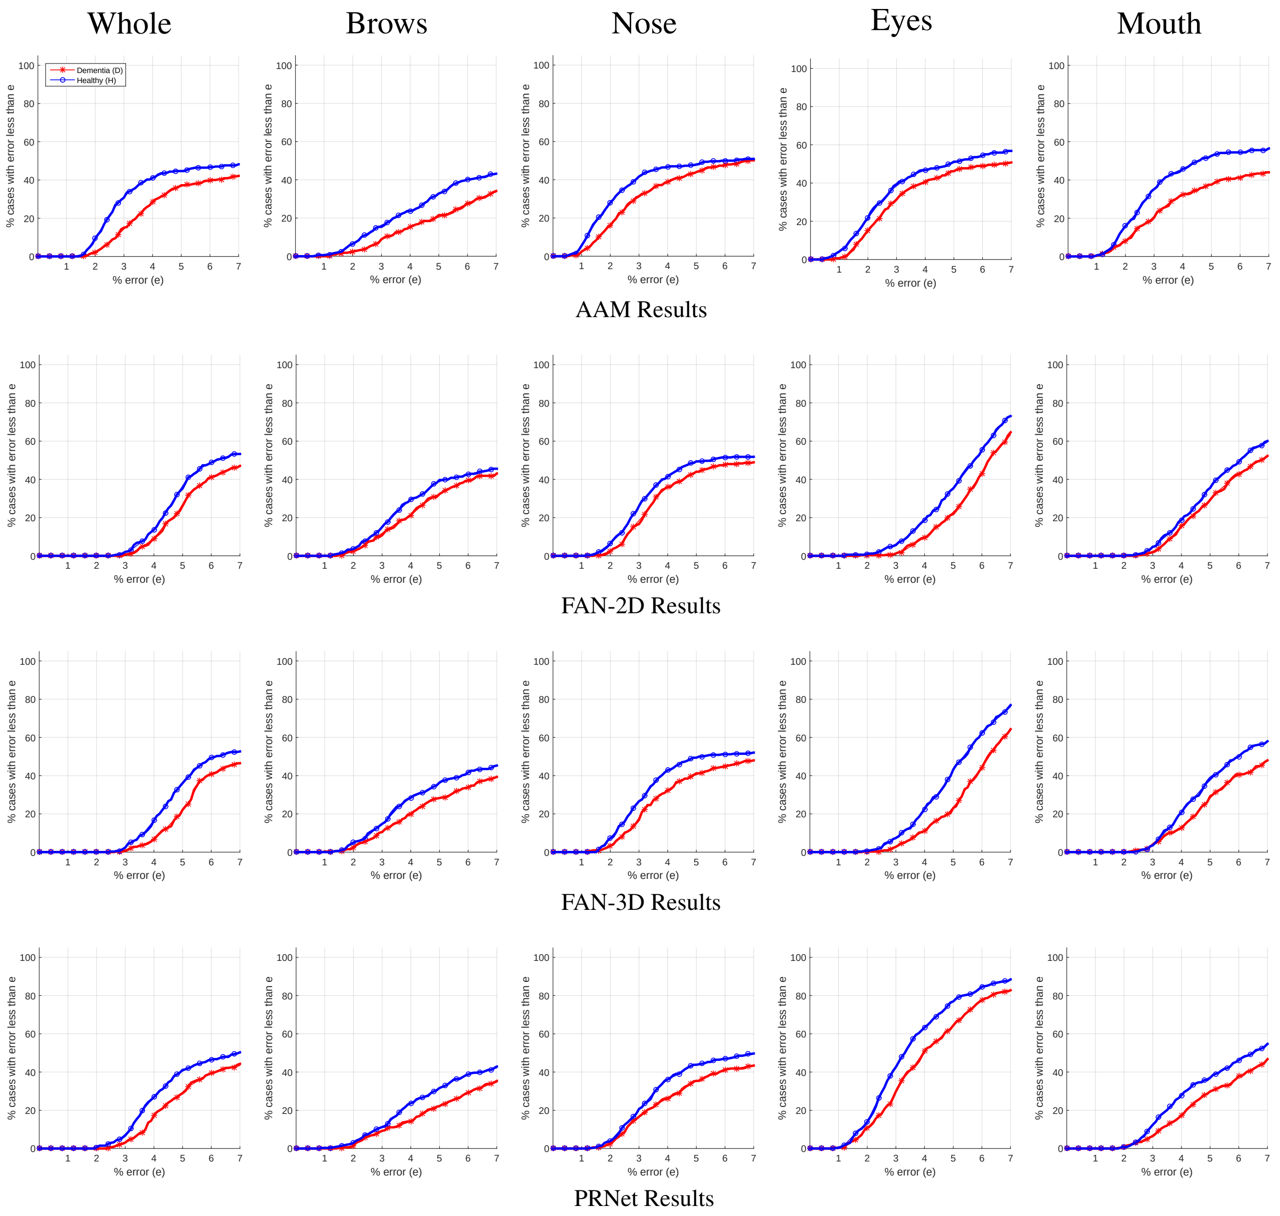


Figure 4: Experiment 4: Comparison of the convergence curves obtained on healthy subset (H) and dementia subset (D) of $T_p$ using four methods: AAM, FAN-2D, FAN-3D, and PRNet.
